# Supplementary material for: Gaussian Harmony: Attaining Fairness in Diffusion-based Face Generation Models
Source: arXiv:2312.14976 source file (2023-12-21)
Supplement: Supplementary file 1 [file X_suppl.tex]

\clearpage
\setcounter{page}{1}
\maketitlesupplementary

% \section{Rationale}
% \label{sec:rationale}
% % 
% Having the supplementary compiled together with the main paper means that:
% % 
% \begin{itemize}
% \item The supplementary can back-reference sections of the main paper, for example, we can refer to \cref{sec:intro};
% \item The main paper can forward reference sub-sections within the supplementary explicitly (e.g. referring to a particular experiment); 
% \item When submitted to arXiv, the supplementary will already included at the end of the paper.
% \end{itemize}
% % 
%  To split the supplementary pages from the main paper, you can use 
%  \href{https://support.apple.com/en-ca/guide/preview/prvw11793/mac#:~:text=Delete%20a%20page%20from%20a,or%20choose%20Edit%20%3E%20Delete).}
%  {Preview (on macOS)}, \href{https://www.adobe.com/acrobat/how-to/delete-pages-from-pdf.html#:~:text=Choose%20%E2%80%9CTools%E2%80%9D%20%3E%20%E2%80%9COrganize,or%20pages%20from%20the%20file.}{Adobe Acrobat} (on all OSs), as well as \href{https://superuser.com/questions/517986/is-it-possible-to-delete-some-pages-of-a-pdf-document}{command line tools}.

% %%%%%%%%%%%%%%%%%%%%%%%%%%%%%%%%%%%%%%%%%%%%%
%  \href{https://support.apple.com/en-ca/guide/preview/prvw11793/mac#:~:text=Delete%20a%20page%20from%20a,or%20choose%20Edit%20%3E%20Delete).}
\section{Introduction}
In this supplementary material, we discuss the rationale behind the effort to mitigate bias in facial generative models, particularly in relation to sensitive attributes like age, gender, and race. Our primary focus is on reducing any potential biases inherent in the unconditional generation of faces by diffusion models, aiming for a more equitable and unbiased representation.

% To begin, we present our findings in the realm of unconditional face generation, utilizing diffusion models. We showcase both successful outcomes and instances where the model falls short, providing a comprehensive overview of its performance.

We also discuss about the Gaussian Mixture Model (GMM) which we add to our reverse diffusion process, elucidating its impact on the separation of distinct classes within each sensitive attribute. This model helps us to achieve a distinction between various attributes such as age groups, genders, and racial categories.

A critical aspect of our approach involves localizing the means of the distributions for each attribute class. By localizing these means, we are able to probabilistically cluster different demographic groups at the latent code level. Subsequently, we sample from these separated noisy codes in such a way that ensures equal representation across attribute classes, effectively mitigating biases introduced during the diffusion model process.

\begin{figure*}
    \centering
    \includegraphics[width = \linewidth]{sec/Supp_FFHQ_Faces.png}
    \caption{Few faces generated by our unconditional diffusion model when trained on FFHQ.}
    \label{ffhq_gen}
\end{figure*}
\begin{figure*}
    \centering
    \includegraphics[width = \linewidth]{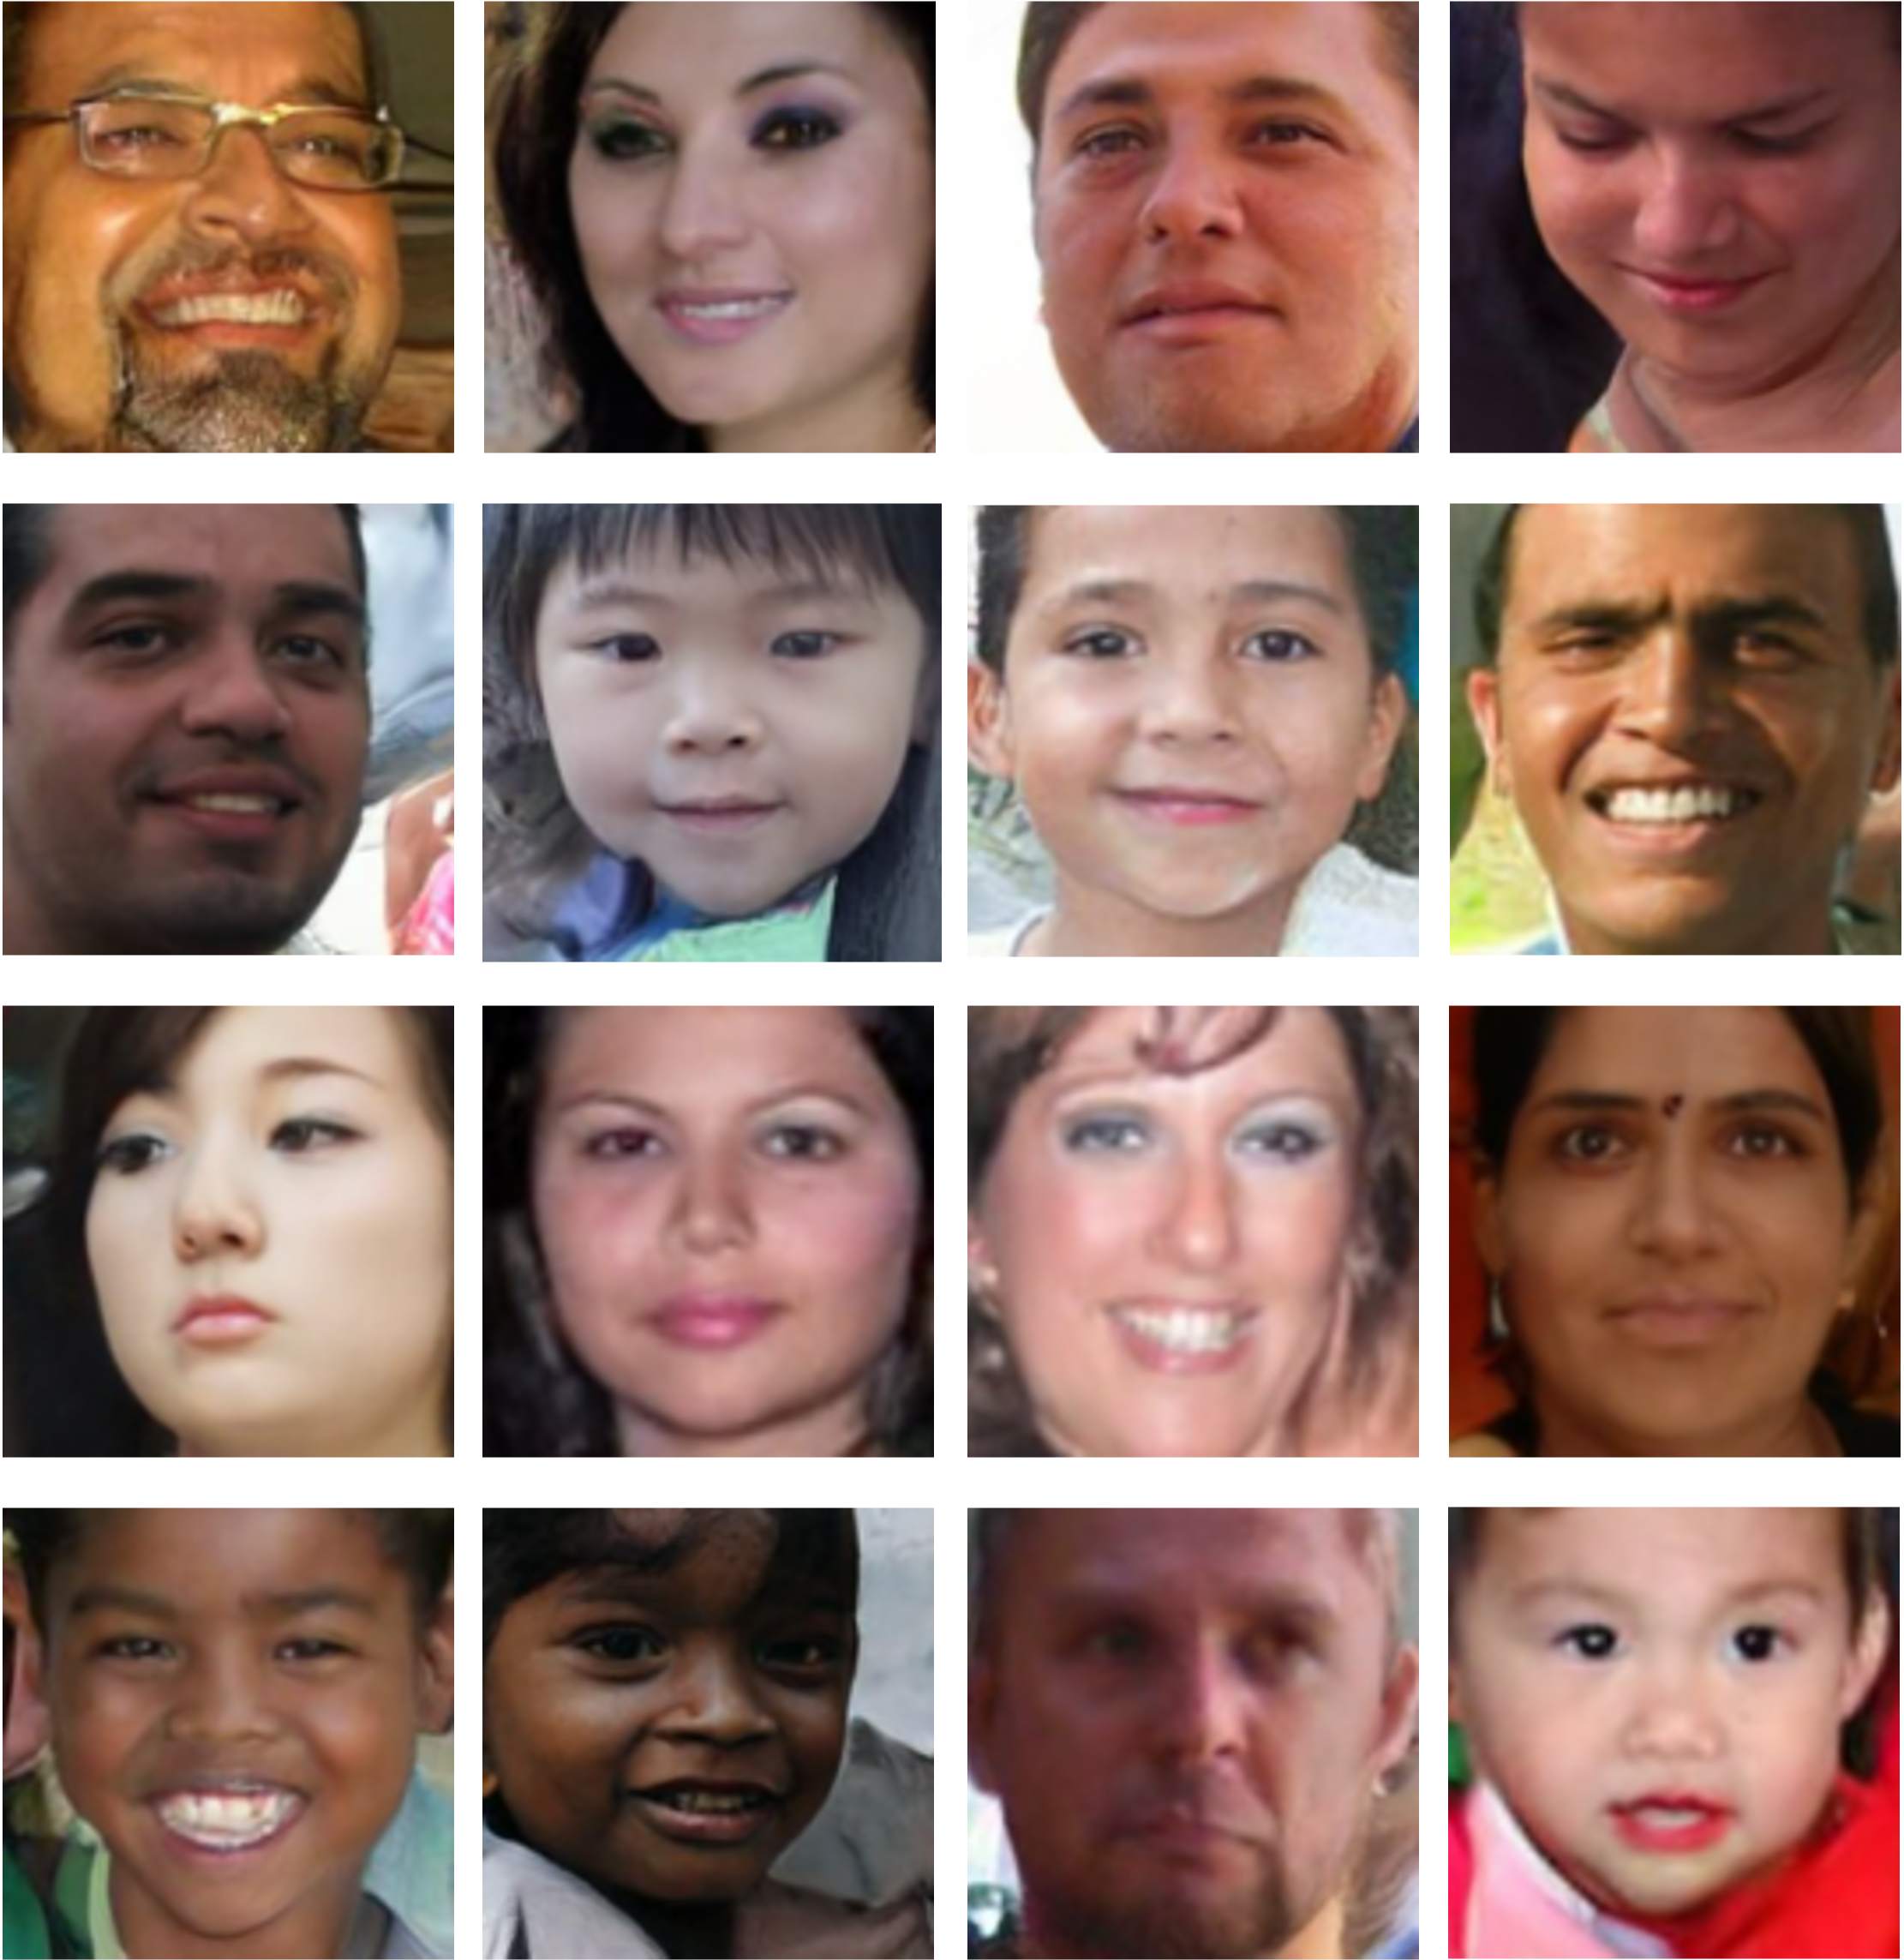}
    \caption{Few faces generated by our unconditional diffusion model when trained on FairFace.}
    \label{ff_gen}
\end{figure*}
\section{Diffusion models for Face Generation}
The use of diffusion model has become widespread for image generation tasks including face generation. We show a few results of our diffusion model on FFHQ and FairFace datasets in Figure \ref{ffhq_gen} and Figure \ref{ff_gen} respectively. The quality of the generated images as seen qualitatively from these figures as well as quantitatively from Table \ref{table1} demonstrate the capacity of diffusion models. However, the major drawback of diffusion models is that it leads to data replication as seen in previous literature especially when it is trained on less data \cite{s1}\cite{s2}. We faced this issue while curating the data for experimenting with training sets balanced in terms of age, gender and race. One potential interpretation for this occurrence is that the complexity of the model surpasses that of the training data, leading to overfitting to the training dataset. For this reason we took the maximum number of images from each class possible even after balancing and did not experiment with smaller balanced datasets.
\section{The Gaussian reasoning}

The rationale behind addressing and mitigating bias related to sensitive attributes such as age, gender, and race in unconditional face generation is rooted in the pursuit of fairness, equity, and ethical considerations. Our motivation is to create generative models that produce diverse and unbiased results, fostering inclusivity and preventing the propagation of unjust societal norms or prejudices. 

In terms of unconditional face generation, bias can be defined as generating more of one class of images than the other. For example: if a trained diffusion model generates more number of male images than female images from noise then it is biased towards male images. For equity, we decide to separate out the classes of sensitive attributes in the latent space itself, so that we can sample equally and finally generate equal number for each class of each attribute. We introduce an approach based on GMMs to address the issue by ensuring a balanced representation of facial attributes in the generated images. We reduce bias through the localization of facial attribute means within the latent space of the diffusion model using these GMMs. The choice of GMMs, as opposed to other clustering frameworks, is motivated by the adaptable latent structure inherent in the diffusion model. Given that each sampling step in diffusion models adhere to a Gaussian distribution, employing a GMM is a plausible and elegant solution to separate out the subspace responsible for generating a specific attribute. Figure \ref{Gaussian_curve_ff} shows the spaces separated out for each of age, gender and race for the FairFace dataset and Figure \ref{Gaussian_curve_FFHQ} shows the same for the FFHQ dataset. This is particularly more efficient as it can be easily integrated as a part of the reverse diffusion process. The results obtained are `bias-corrected' without any retraining.
